# Supplementary material for: Strong coupling quantum electrodynamics Hartree-Fock response theory
Source: arXiv:2502.14511 source file (2025-02-20)
Supplement: Supplementary file 1 [file SI.pdf]

# Supporting Information – Strong coupling quantum electrodynamical Hartree-Fock response theory: a simple analysis of electron-photon correlation

Matteo Castagnola,<sup>†</sup> Rosario R. Riso,<sup>†</sup> Yassir El Moutaoukal,<sup>†</sup> Enrico Ronca,<sup>‡</sup>  
and Henrik Koch<sup>\*,†</sup>

<sup>†</sup>*Department of Chemistry, Norwegian University of Science and Technology, 7491  
Trondheim, Norway*

<sup>‡</sup>*Dipartimento di Chimica, Biologia e Biotecnologie, Università degli Studi di Perugia, Via  
Elce di Sotto, 8, 06123, Perugia, Italy*

E-mail: henrik.koch@ntnu.no

## 1 Theory

In this section, we provide analytical proof that the TD-SC-QED-HF model fulfills the equivalence relations

$$\omega_n \langle 0|q|n \rangle = i \langle 0|p|n \rangle \quad (1)$$

and

$$\omega_n \langle 0|\mathbf{r}_i|n \rangle = i \langle 0|\mathbf{p}_i|n \rangle. \quad (2)$$

To this end, we prove that the first-order equation of motion<sup>1,2</sup>

$$\omega_1 \langle\langle A; V^{\omega_1} \rangle\rangle_{\omega_1} = \langle\langle [A, H]; V^{\omega_1} \rangle\rangle_{\omega_1} + \langle 0 | [A, V^{\omega_1}] | 0 \rangle \quad (3)$$

is fulfilled.<sup>3</sup> Consider the relation

$$iP = [Q, H], \quad (4)$$

and we want to prove that

$$\langle\langle P; V^{\omega_1} \rangle\rangle_{\omega_1} = -i\omega_1 \langle\langle Q; V^{\omega_1} \rangle\rangle_{\omega_1} + i \langle 0 | [A, V^{\omega_1}] | 0 \rangle. \quad (5)$$

The response function for the operator  $P$  is

$$\begin{aligned} \langle\langle P, V \rangle\rangle_{\omega_1+i\epsilon} &= \frac{1}{\sqrt{2}} \sum_{ai} \kappa_{ai}^{\omega_1} \langle\langle [Q_X, H_X], E_{ai} \rangle\rangle_R + \frac{1}{\sqrt{2}} \sum_{ai} \kappa_{ia}^{-\omega_1} \langle\langle [Q_X, H_X], E_{ia} \rangle\rangle_R \\ &\quad + \gamma^{\omega_1} \langle\langle [Q_X, H_X], b^\dagger \rangle\rangle_R + \gamma^{-\omega_1} \langle\langle [Q_X, H_X], b \rangle\rangle_R \end{aligned} \quad (6)$$

where  $Q_X = U_X^\dagger Q U_X$  is the operator transformed with the ground state SC-QED-HF transformation, and the same is valid for the Hamiltonian  $H_X$ . The average value is then computed for the reference state

$$|R\rangle = |\text{HF}\rangle \otimes |0\rangle. \quad (7)$$

Notice that, for the electric dipole operator  $Q = \mathbf{d}$  (for a complete basis set) and for the photon momentum  $p$  we have

$$\mathbf{d}_X = U_X^\dagger \mathbf{d} U_X = \mathbf{d} \quad p_X = U_X^\dagger p U_X = p, \quad (8)$$

while for the photon coordinate

$$q_X = U_X^\dagger q U_X = \frac{b + b^\dagger}{\sqrt{2\omega}} + \frac{2}{\omega} \frac{1}{\sqrt{2\omega}} \sum_p \eta_p \tilde{E}_{pp}. \quad (9)$$

First, consider a one-electron operator  $Q$

$$Q = \frac{1}{\sqrt{2}} \sum_{ai} (Q_{ai} E_{ai} + Q_{ai}^* E_{ia}) + \delta Q \quad (10)$$

where  $\delta Q$  includes only the redundant electronic operators  $E_{ab}$  and  $E_{ij}$

$$\delta Q = \frac{1}{\sqrt{2}} \sum_{ab} Q_{ab} E_{ab} + \frac{1}{\sqrt{2}} \sum_{ij} Q_{ij} E_{ij} \quad (11)$$

where  $a$  and  $b$  refer to virtual orbitals while  $i$  and  $j$  to occupied orbitals in Eq. 7. Taking  $Q$  to be a component of the electric dipole operator, we can substitute  $Q_X$  with  $Q$  in the response function (in the complete basis approximation) to obtain

$$\begin{aligned} \langle \langle P, V \rangle \rangle_{\omega_1 + i\epsilon} &= \frac{1}{2} \sum_{aibj} \kappa_{ai}^{\omega_1} \langle [[Q_{bj} E_{bj} + Q_{bj}^* E_{jb}, H_X], E_{ai}] \rangle_R + \frac{1}{2} \sum_{aibj} \kappa_{ia}^{-\omega_1} \langle [[Q_{bj} E_{bj} + Q_{bj}^* E_{jb}, H_X], E_{ia}] \rangle_R \\ &+ \frac{1}{\sqrt{2}} \sum_{ai} \kappa_{ai}^{\omega_1} \langle [[\delta Q, H_X], E_{ai}] \rangle_R + \frac{1}{\sqrt{2}} \sum_{ai} \kappa_{ia}^{-\omega_1} \langle [[\delta Q, H_X], E_{ia}] \rangle_R \\ &+ \frac{1}{\sqrt{2}} \sum_{\alpha bj} \gamma_{\alpha}^{\omega_1} \langle [[Q_{bj} E_{bj} + Q_{bj}^* E_{jb}, H_X], b_{\alpha}^{\dagger}] \rangle_R + \frac{1}{\sqrt{2}} \sum_{\alpha bj} \gamma_{\alpha}^{-\omega_1} \langle [[Q_{bj} E_{bj} + Q_{bj}^* E_{jb}, H_X], b_{\alpha}] \rangle_R \\ &+ \sum_{\alpha} \gamma_{\alpha}^{\omega_1} \langle [[\delta Q, H_X], b_{\alpha}^{\dagger}] \rangle_R + \sum_{\alpha} \gamma_{\alpha}^{-\omega_1} \langle [[\delta Q, H_X], b_{\alpha}] \rangle_R \\ &= \begin{pmatrix} 0 & Q_{ai}^* & 0 & Q_{ai} \end{pmatrix} \begin{pmatrix} \mathbf{A} & \mathbf{B} \\ \mathbf{B}^* & \mathbf{A}^* \end{pmatrix} \begin{pmatrix} \gamma^{\omega_1} \\ \kappa_{ai}^{\omega_1} \\ \gamma^{-\omega_1} \\ \kappa_{ia}^{-\omega_1} \end{pmatrix} \\ &+ \frac{1}{\sqrt{2}} \sum_{ai} \kappa_{ai}^{\omega_1} \langle [[\delta Q, H_X], E_{ai}] \rangle_R + \frac{1}{\sqrt{2}} \sum_{ai} \kappa_{ia}^{-\omega_1} \langle [[\delta Q, H_X], E_{ia}] \rangle_R \\ &+ \sum_{\alpha} \gamma_{\alpha}^{\omega_1} \langle [[\delta Q, H_X], b_{\alpha}^{\dagger}] \rangle_R + \sum_{\alpha} \gamma_{\alpha}^{-\omega_1} \langle [[\delta Q, H_X], b_{\alpha}] \rangle_R \end{aligned}$$

Now we can write, by using Jacobi's identity

$$\begin{aligned}
&= \begin{pmatrix} 0 & Q_{ai}^* & 0 & Q_{ai} \end{pmatrix} \begin{pmatrix} \mathbf{A} & \mathbf{B} \\ \mathbf{B}^* & \mathbf{A}^* \end{pmatrix} \begin{pmatrix} \gamma^{\omega_1} \\ \kappa_{ai}^{\omega_1} \\ \gamma^{-\omega_1} \\ \kappa_{ia}^{-\omega_1} \end{pmatrix} \\
&\quad - \sum_{ai} \kappa_{ai}^{\omega_1} \langle [[E_{ai}, \delta Q], H_X] \rangle_R - \sum_{ai} \kappa_{ai}^{-\omega_1} \langle [[H_X, E_{ai}], \delta Q] \rangle_R \\
&\quad - \sum_{ai} \kappa_{ia}^{\omega_1} \langle [[E_{ia}, \delta Q], H_X] \rangle_R - \sum_{ai} \kappa_{ia}^{-\omega_1} \langle [[H_X, E_{ia}], \delta Q] \rangle_R \\
&\quad - \sum_{\alpha} \gamma_{\alpha}^{\omega_1} \langle [[b_{\alpha}^{\dagger}, \delta Q], H_X] \rangle_R - \sum_{\alpha} \gamma_{\alpha}^{-\omega_1} \langle [[H_X, b_{\alpha}], \delta Q] \rangle_R \\
&\quad - \sum_{\alpha} \gamma_{\alpha}^{\omega_1} \langle [[b_{\alpha}^{\dagger}, \delta Q], H_X] \rangle_R - \sum_{\alpha} \gamma_{\alpha}^{-\omega_1} \langle [[H_X, b_{\alpha}], \delta Q] \rangle_R.
\end{aligned}$$

When  $\delta Q$  is applied on the reference eave function, the result is either zero or the same (rescaled) HF wave function, so the right commutators in the last four lines are identically zero. Then,  $\delta Q$  commutes with  $b^{\dagger}$ , so the last two lines are identically zero. Finally, if we compute the commutator between  $\delta O$  and  $E_{ai}$  or  $E_{ia}$  we get

$$\begin{aligned}
[E_{lm}, E_{ai}] &= E_{li}\delta_{am} - E_{am}\delta_{il} \\
[E_{cd}, E_{ia}] &= E_{ca}\delta_{di} - E_{id}\delta_{ac}
\end{aligned} \tag{12}$$

so the first terms of the first two lines are zero either because of the deltas in 12 or because of the generalized Brillouin's theorem. We are thus left only with the first line, and from the

response equation we obtain

$$\begin{aligned}
&= \begin{pmatrix} 0 & O_{ai}^* & 0 & O_{ai} \end{pmatrix} \left[ i \begin{pmatrix} \langle [b, V^{\omega_1}] \rangle_R \\ \frac{1}{\sqrt{2}} \langle [E_{ja}, V^{\omega_1}] \rangle_R \\ \langle [b^\dagger, V^{\omega_1}] \rangle_R \\ \frac{1}{\sqrt{2}} \langle [E_{aj}, V^{\omega_1}] \rangle_R \end{pmatrix} + \omega_1 \begin{pmatrix} 1 & 0 & 0 & 0 \\ 0 & 1 & 0 & 0 \\ 0 & 0 & -1 & 0 \\ 0 & 0 & 0 & -1 \end{pmatrix} \begin{pmatrix} \gamma^{\omega_1} \\ \kappa_{ai}^{\omega_1} \\ \gamma^{-\omega_1} \\ \kappa_{ia}^{-\omega_1} \end{pmatrix} \right] \\
&= i \langle [O, V^{\omega_1}] \rangle_R + \omega_1 (O_{ia} \kappa_{ai}^{\omega_1} - O_{ai} \kappa_{ia}^{-\omega_1}) \\
&= i \langle [O, V^{\omega_1}] \rangle_R + \omega_1 \frac{1}{\sqrt{2}} \left( \langle [O, E_{ai}] \rangle_R \kappa_{ai}^{\omega_1} + \langle [O, E_{ia}] \rangle_R \kappa_{ia}^{-\omega_1} \right), \tag{13}
\end{aligned}$$

which is precisely the equation of motion Eq. 3 for the linear response. This relation ensures the equivalence between the dipole and velocity formulation for the transition moments

$$\omega_n \langle 0 | \mathbf{r}_i | n \rangle = i \langle 0 | \mathbf{p}_i | n \rangle. \tag{14}$$

A similar proof holds for the photon relation

$$\omega_n \langle 0 | q | n \rangle = i \langle 0 | p | n \rangle. \tag{15}$$

In this case, from Eq. 9 we write

$$Q_X = \frac{1}{\sqrt{2}} \sum_{ai} (Q_{ai} E_{ai} + Q_{ai}^* E_{ia}) + \delta Q + \frac{b + b^\dagger}{\sqrt{2}\omega} \tag{16}$$

and obtain

$$\begin{aligned}
\langle\langle P, V \rangle\rangle_{\omega_1+i\epsilon} &= \frac{1}{2} \sum_{aibj} \kappa_{ai}^{\omega_1} \langle [[Q_{bj}E_{bj} + Q_{bj}^*E_{jb} + \frac{b+b^\dagger}{\sqrt{\omega}}, H_X], E_{ai}] \rangle_R \\
&+ \frac{1}{2} \sum_{aibj} \kappa_{ia}^{-\omega_1} \langle [[Q_{bj}E_{bj} + Q_{bj}^*E_{jb} + \frac{b+b^\dagger}{\sqrt{\omega}}, H_X], E_{ia}] \rangle_R \\
&+ \frac{1}{\sqrt{2}} \sum_{ai} \kappa_{ai}^{\omega_1} \langle [[\delta Q, H_X], E_{ai}] \rangle_R + \frac{1}{\sqrt{2}} \sum_{ai} \kappa_{ia}^{-\omega_1} \langle [[\delta Q, H_X], E_{ia}] \rangle_R \\
&+ \frac{1}{\sqrt{2}} \sum_{\alpha bj} \gamma_\alpha^{\omega_1} \langle [[Q_{bj}E_{bj} + Q_{bj}^*E_{jb} + \frac{b+b^\dagger}{\sqrt{\omega}}, H_X], b_\alpha^\dagger] \rangle_R \\
&+ \frac{1}{\sqrt{2}} \sum_{\alpha bj} \gamma_\alpha^{-\omega_1} \langle [[Q_{bj}E_{bj} + Q_{bj}^*E_{jb} + \frac{b+b^\dagger}{\sqrt{\omega}}, H_X], b_\alpha] \rangle_R \\
&+ \sum_\alpha \gamma_\alpha^{\omega_1} \langle [[\delta Q, H_X], b_\alpha^\dagger] \rangle_R + \sum_\alpha \gamma_\alpha^{-\omega_1} \langle [[\delta Q, H_X], b_\alpha] \rangle_R \\
&= \begin{pmatrix} \frac{1}{\sqrt{2\omega}} & Q_{ai}^* & \frac{1}{\sqrt{2\omega}} & Q_{ai} \end{pmatrix} \begin{pmatrix} \mathbf{A} & \mathbf{B} \\ \mathbf{B}^* & \mathbf{A}^* \end{pmatrix} \begin{pmatrix} \gamma^{\omega_1} \\ \kappa_{ai}^{\omega_1} \\ \gamma^{-\omega_1} \\ \kappa_{ia}^{-\omega_1} \end{pmatrix} \\
&+ \frac{1}{\sqrt{2}} \sum_{ai} \kappa_{ai}^{\omega_1} \langle [[\delta Q, H_X], E_{ai}] \rangle_R + \frac{1}{\sqrt{2}} \sum_{ai} \kappa_{ia}^{-\omega_1} \langle [[\delta Q, H_X], E_{ia}] \rangle_R \\
&+ \sum_\alpha \gamma_\alpha^{\omega_1} \langle [[\delta Q, H_X], b_\alpha^\dagger] \rangle_R + \sum_\alpha \gamma_\alpha^{-\omega_1} \langle [[\delta Q, H_X], b_\alpha] \rangle_R.
\end{aligned}$$

Following the same reasoning as above, we obtain the same equation of motion for the linear response function, and thus the equivalence between the transition moments of the photon coordinate and momentum

$$\omega_n \langle 0|q|n \rangle = i \langle 0|p|n \rangle. \quad (17)$$

Notice that in this case, we do not need a complete basis set since the commutator relation

$$[b, b^\dagger] = 1 \quad (18)$$

is fulfilled independently of the basis set size, and the equations are not solved in a truncated photon subspace space. The same proof clearly also holds for TD-QED-HF.<sup>3</sup>

## 2 Molecular Geometries

Table 1: Molecular geometry of the formaldehyde molecule. The coordinates are given in Angstrom Å

|   | Atom | x [Å]           | y [Å]          | z [Å]           |
|---|------|-----------------|----------------|-----------------|
| 1 | H    | -0.945037072500 | 0.000000000000 | 1.128390875700  |
| 2 | C    | 0.000000000000  | 0.000000000000 | 0.526758766300  |
| 3 | H    | 0.945037072500  | 0.000000000000 | 1.128390875700  |
| 4 | O    | 0.000000000000  | 0.000000000000 | -0.677166793600 |

Table 2: Molecular geometry of the para-nitroaniline molecule. The coordinates are given in Angstrom Å

|    | Atom | x [Å]           | y [Å]           | z [Å]          |
|----|------|-----------------|-----------------|----------------|
| 1  | N    | -2.157464580000 | 0.000000000000  | 0.000000000000 |
| 2  | C    | -0.703214720000 | 0.000000000000  | 0.000000000000 |
| 3  | C    | -0.011457210000 | 1.216931100000  | 0.000000000000 |
| 4  | H    | -0.567736250000 | 2.146975030000  | 0.000000000000 |
| 5  | C    | 1.374820520000  | 1.216566830000  | 0.000000000000 |
| 6  | H    | 1.914253020000  | 2.160555050000  | 0.000000000000 |
| 7  | C    | 2.095469890000  | 0.000000000000  | 0.000000000000 |
| 8  | N    | 3.466119360000  | 0.000000000000  | 0.000000000000 |
| 9  | H    | 3.990101500000  | 0.861405000000  | 0.000000000000 |
| 10 | H    | 3.990101500000  | -0.861405000000 | 0.000000000000 |
| 11 | C    | 1.374820520000  | -1.216566830000 | 0.000000000000 |
| 12 | H    | 1.914253020000  | -2.160555050000 | 0.000000000000 |
| 13 | C    | -0.011457210000 | -1.216931100000 | 0.000000000000 |
| 14 | H    | -0.567736250000 | -2.146975030000 | 0.000000000000 |
| 15 | O    | -2.739659740000 | 1.091436200000  | 0.000000000000 |
| 16 | O    | -2.739659740000 | -1.091436200000 | 0.000000000000 |

Table 3: Molecular geometry of the fluoridic acid. The coordinates are given in Angstrom Å

|   | Atom | x [Å]          | y [Å]          | z [Å]          |
|---|------|----------------|----------------|----------------|
| 1 | H    | 0.000000000000 | 0.000000000000 | 0.000000000000 |
| 2 | F    | 0.916800000000 | 0.000000000000 | 0.000000000000 |

## References

- (1) Olsen, J.; Jørgensen, P. Linear and nonlinear response functions for an exact state and for an MCSCF state. *The Journal of chemical physics* **1985**, *82*, 3235–3264.
- (2) Dalgaard, E. Time-dependent multiconfigurational Hartree–Fock theory. *The Journal of Chemical Physics* **1980**, *72*, 816–823.
- (3) Castagnola, M.; Riso, R. R.; Barlini, A.; Ronca, E.; Koch, H. Polaritonic response theory for exact and approximate wave functions. *Wiley Interdisciplinary Reviews: Computational Molecular Science* **2024**, *14*, e1684.
